# Supplementary material for: Logarithmic series and Hodge integrals in the tautological ring (with an appendix by D. Zagier)
Source: arXiv:math/0002112 source file (2000-03-09)
Supplement: Supplementary file 1 [file logappendix.tex]

\input amstex
\documentstyle{amsppt} \magnification=\magstephalf \parskip=4pt \nologo 
\hsize=6true in \vsize=9true in \NoBlackBoxes \NoRunningHeads  \TagsOnRight
    \def\Q{\Bbb Q} \def\N{\Bbb N}  \def\Z{\Bbb Z} 
\def\a{\alpha} \def\b{\beta} \def\g{\gamma} \def\l{\lambda}  
\def\={\;=\;} \def\:{\;:=\;}  \def\-{\,-\,}  \def\+{\,+\,}
\def\C#1{\Cal C\bigl(#1\bigr)} \def\B{\Cal B} \def\B{\Cal B} \def\wB{\widehat B}  \def\P{\frak P} \def\tQ{\widetilde Q}
\def\bb#1{\noindent{\bf #1.}} \def\q{\quad} \def\qq{\qquad} \def\bs{\blacksquare} \def\endpf{$\q\bs$} 

\topmatter\title Appendix: Polynomials arising from the tautological ring \endtitle
\author Don Zagier\endauthor\endtopmatter

{\bf 1. Statement of results.} For positive integers $g$ and $k$ define
 $$ P_g(k)\=\sum_{l=1}^k\frac{(k-1)!}{(k-l)!}\,\frac1{k^l}\,\sum_{m=1}^l(-1)^{l-m}\binom lm\frac{m^{2g+l-1}}{(2g+l-1)!}\tag 1$$
(the inner sum here is a Stirling number), e.g.~for $k\le3$,
  $$P_g(1)\=\frac1{(2g)!}\,,\q P_g(2)\=\frac{2^{2g-1}+g}{(2g+1)!}\,,\q P_g(3)\=\frac{2(3^{2g+1}+2^{2g+2}g+6g^2+5g)}{9(2g+2)!}\,.$$
A property of the function $P_g$ which is far from obvious---and is false if the number $2g-1$ on the right-hand side of (1) is replaced
by an even number---is that it is a polynomial in~$k$ for each fixed $g$, the first values being
$$ P_1(k)=\frac12\,,\;\q P_2(k)=\frac k{24}\,,\;\q P_3(k)=\frac{3k^2-k}{1440}\,,\;\q P_4(k)=\frac{9k^3-8k^2+2k}{120960}\,.$$
This fact was discovered and proved in the preceding article [1] by Faber and Pandharipande by an indirect argument in which the coefficients
of the polynomials $P_g(k)$ were interpreted as intersection numbers of certain cycles in the moduli space of curves of genus~$g$. 
Here we will give a more direct combinatorial proof and will also obtain alternative expressions for the polynomial $P_g(k)$ and 
explicit formulas for its highest and lowest coefficients.  The formulas for the coefficients of $k^{g-1}$, $k^{g-2}$, $k^2$ 
and $k^1$ were quoted in Section 5.2 of [1].
\proclaim{Theorem 1} (i)\ For each integer $g\ge1$, the function $P_g(k)$ defined by $(1)$ is a polynomial of degree $g-1$ in $k$.
\smallskip \noindent
(ii)\ Write $P_g(k)=\sum_{i=0}^{g-1}c_{g,i}k^i\,$.  Then for fixed $j\ge0$ and $g>j$ we have
$$ c_{g,g-j-1} \= \frac{(g-1)!}{2^g\,(2g-1)!}\,C_j(g)\,,\tag 2$$
where  
 $$ C_0(g)=1,\q C_1(g)=-\frac{g(g-2)}9\,,\q C_2(g)=\frac{g(g-3)(5g^2-9g+1)}{810}\,,$$
and in general $C_j(g)$ is a polynomial of degree $2j$  with leading coefficient $\dfrac{(-1/9)^j}{j!}\,$.
\smallskip \noindent
(iii)\ For fixed $i\ge0$ and $g>i+1$ we have $c_{g,i}=\sum\limits_{j=0}^{i}\g_{i,j}(g)\,\b_{2g-j-1},$  where 
$\b_n=\dfrac{B_n}{n!}$ $(B_n$ = $n$th Bernoulli number$)$ and $\g_{i,j}(g)$ is a polynomial of degree $i-j$. In particular $($for $g>2)$ 
$$ c_{g,0}= 0\,,\q c_{g,1} = \frac12\,\b_{2g-2}\,,\q c_{g,2} =\,-\frac g2\,\b_{2g-2}\,,\q
c_{g,3} =\frac{g(g+2)}6\,\b_{2g-2}+\frac1{24}\,\b_{2g-4}\,.$$ 
\endproclaim
\newpage
Parts (i) and (ii) of Theorem~1 are equivalent to the following amusing result. Let us define numbers $A(g,n)$ ($g\ge1,\,n\ge0$) by
$$ \sum_{n=0}^\infty A(g,n)\,x^n = e^{-x}\,\sum_{k=0}^\infty P_g(k)\,\frac{x^k}{k!} $$
or equivalently by
$$  A(g,n)\=\sum_{k=0}^n\,\frac{(-1)^{n-k}}{k!\,(n-k)!}\,P_g(k)\,,\qq P_g(k)\=\sum_{n=0}^k\,\frac{k!}{(k-n)!}\,A(g,n)\,.\tag 3$$
\proclaim{Theorem 2} The numbers $A(g,n)$ vanish for $n\ge g$. For $n\le g-1$ we have
$$ A(g,n)\=\frac{(g-1)!}{2^g\,(2g-1)!}\,C^*_{g-n-1}(g-n-1)\,,\tag 4$$
where
  $$ C^*_0(h)=1\,,\q C^*_1(h)=\frac{7h^2+5h}{18}\,,\q C^*_2(h)=\frac{245h^4+594h^3+283h^2-42h}{3240}\,,$$
and in general $C^*_r(h)$ is a polynomial of degree $2r$ in $h$ with leading coefficient $\dfrac{(7/18)^r}{r!}\,$.
\endproclaim
\noindent This theorem, as well as more general results concerning the numbers
$$  A_\nu(g,n)\=\sum_{k=1}^n\,\frac{(-1)^{n-k}}{k!\,(n-k)!}\,k^{-\nu}\,P_g(k)\qq (\nu\ge0), $$
which are related to part (iii) of Theorem~1, will be proved in \S3. For instance, we have
$$ A_1(g,n)= \frac{(-1)^{n-1}}{2\,n!}\,\b_{2g-2}\,,\q\; A_2(g,n)=A_1(g,n)\,\bigl(g-\sum_{k=1}^n\frac1k\bigr)\qq(n+2\ge g>2).  \tag 5 $$

To state the remaining results, and for the proofs, we will need some more notation.  As in [1], we write $\C{x^n,f(x)}$ to
denote the coefficient of $x^n$ in a power series $f(x)$ and $h_n(\a_1,\ldots,\a_l)=\C{x^n,\prod_{i=1}^l(1-\a_ix)^{-1}}$ for
the full symmetric function of degree $n$ in variables $\a_1,\ldots,\a_l$. For any integer $n\ge0$, we define $S_n(l)$ by
  $$ S_n(l) \= \C{x^n,\,\bigl(\frac{e^x-1}x\bigr)^l}\,. \tag 6$$
For $l\in\N$ we have the formulas
 $$\frac{(n+l)!}{l!}\,S_n(l)\=\frac1{l!}\sum_{m=0}^l(-1)^{l-m}\binom lmm^{n+l}
   \=h_n\bigl(1,\,2,\ldots,\,l\bigr) \=\frak S^{(l)}_{n+l}\,, $$
where $\frak S^{(l)}_{n+l}$ denotes the Stirling number of the second kind (=number of partitions of a 
set of $n+l$ elements into $l$ non-empty subsets).  In particular, equation~(1) can be written
 $$ P_g(k)\=\sum_{l=1}^k\frac{(k-1)!}{(k-l)!}\,\frac1{k^l}\,S_{2g-1}(l)\,.\tag 7$$
However, $S_n(l)$ is a polynomial (of degree $n$) in $l$, the first values being 
  $$ S_0(l)\=1,\q S_1(l)\=\frac l2\,,\q S_2(l)=\frac{3l^2+l}{24}\,,\q S_3(l)=\frac{l^3+l^2}{48}\,,\;\ldots,$$
so it makes sense for any complex value of $l$. For $l=0$ we clearly have $S_n(l)=0$ for all $n>0$. For $l=-1$ we have
$S_n(l)=\b_n$ by definition, where $\b_n=B_n/n!$ as in Theorem~1, and more generally $S_n(l)$ for fixed negative $l$
is a finite combination of Bernoulli numbers (Lemma 3 below), the first three cases for $n$ odd being
  $$ S_{2g-1}(-1)=0,\q S_{2g-1}(-2)=-\b_{2g-2}\,,\q S_{2g-1}(-3)=\frac32\,(2g-3)\,\b_{2g-2}\qq(g\ge3).$$
Using these numbers, we can now state a formula for $P_g(t)$ as a power series in $t$.  
\proclaim{Theorem 3} Define the function $S_n(l)$ by eq.~$(6)$.  Then for each integer $g\ge1$ we have 
$$ P_g(t)\=-\,\sum_{r=1}^\infty\frac{S_{2g-1}(-r)\,t^{r-1}}{(1+t)\cdots(r+t)} \qq\in\;\Q[[t]]\;. \tag 8$$
In particular, the power series on the right-hand side of $(8)$ is in fact a polynomial in $t$.\endproclaim
\noindent This theorem gives an alternative definition of the polynomials $P_g(t)$, but, as with~(1), the polynomial property is 
not clear from this definition, and is not true if the index $2g-1$ on the right-hand side of (8) is replaced by an even number.

The next result gives a closed form expression for the generating function of the $P_g(t)$ as an integral. This looks less 
elementary than the preceding results, but has the advantage of making it obvious that $P_g$ is a polynomial. 
\proclaim{Theorem 4}  Define a power series $F(x)$ by
   $$  \align F(x)&\=\frac{\sinh x/2}{x/2}\,\exp\biggl(\frac{x/2}{\tanh x/2}-1\biggr)
   \=\exp\biggl(\sum_{n=2}^\infty\frac{n+1}n\,\b_n\,x^n\biggr) \tag 9\\   
   &\=1\+\frac18\,x^2\+\frac7{1152}\,x^4\+\frac{61}{414720}\,x^6\,+\;\cdots\;.\endalign $$
Then the $P_g(t)$ are given by the generating function identity
   $$  \sum_{g=1}^\infty P_g(t)\,x^{2g-1}\=\frac12\,F(x)^t\int_0^x F(y)^{-t}\,dy\,.\tag 10$$ 
\endproclaim \noindent 
The polynomiality of the functions $P_g(t)$ follows immediately because we can rewrite the generating series identity (10) in the form
$$ P_g(t)\=\sum_{n=0}^{g-1}\frac{p_{g-1-n}(t)\,p_n(-t)}{2(2n+1)}\,,$$
where $p_n(t)$ denotes the coefficient of $x^{2n}$ in $F(x)^t$, which is clearly a polynomial in $t$ of degree $n$.
Equation~(10) is also equivalent to the following recursion for the polynomials $P_g$.
\proclaim{Theorem 5} The polynomials $P_g(t)$ can be given recursively by the formulas
$$  P_1(t)=\frac12\,,\qq P_g(t)\=\frac t{2g-1}\,\sum_{n=1}^{g-1} (2n+1)\,\beta_{2n}\,P_{g-n}(t)\qq(g\ge2)\,.\tag11$$
\endproclaim

The final result describes the coefficients $c_{g,i}$ (which are actually the numbers of interest, since it is they, and
not the values of the polynomial $P_g(k)$, which occur in [1] as intersection numbers) via a generating series with
respect to the variable $g$ rather than $i$.  We begin with the well-known fact that the inverse power series of $x=ye^{-y}$ is
given by $y=\sum_{k\ge1} k^{k-1}x^k/k!\,$.  A simple generalization of this says that the power series
  $$ Q_i(y)\=(-1)^i\sum_{k=1}^\infty\frac{k^{k-1-i}}{k!}\,(ye^{-y})^k \tag12$$
is in fact a polynomial in $y$ for every integer $i\ge0$, the first few values being
  $$ Q_0(y)=y,\;\,Q_1(y)=\frac12y^2-y,\;\,Q_2(y)=\frac16y^3-\frac34y^2+y,\;\,Q_3(y)=\frac1{24}y^4-\frac{11}{36}y^3+\frac78y^2-y\,.$$
The polynomials $Q_i(y)$ can also be defined and computed using the recursion 
  $$ Q_0(y)=y,\qq Q_{i+1}(y)=\int_0^y\frac{x-1}x\,Q_i(x)\,dx \qq(i\ge0)\tag13$$
or the generating function identity
  $$ \sum_{i=0}^\infty Q_i(y)\,t^i=\sum_{r=1}^\infty\frac{t^{r-1}y^r} {(1+t)\cdots(r+t)}\,. \tag14 $$
The following theorem provides yet another characterization of these polynomials and a new generating function for the 
rational numbers $c_{g,i}\,$.
\proclaim{Theorem 6} (i)\ The polynomial $Q_i$ is, up to a constant, the unique polynomial  with
constant term~$0$ and degree $\le i+1$ satisfying
 $$ Q_i\bigl(\frac x{1-e^{-x}}\bigr)- Q_i\bigl(\frac x{e^x-1}\bigr)=\text O\bigl(x^{2i+1}\bigr)\qq\qq (x\to0)\,. \tag15$$
\smallskip \noindent
(ii)\ For all integers $g\ge1$ and $i\ge0$ we have
    $$c_{g,i\,}\=\C{x^{2g-1},\,Q_i\bigl(\frac x{1-e^{-x}}\bigr)}\,. \tag16 $$  \endproclaim

The proof of this theorem will be given in \S5.

\bigskip {\bf 2. Polynomials defined by functional equations.}
We begin by giving two simple (and well-known) lemmas which will be used several times in the sequel.
\proclaim{Lemma 1} Let $r$ be a non-negative integer and $z$ be a variable.  Then
  $$\frac1{z(z-1)\cdots(z-r)}\=\sum_{m=0}^r\frac{(-1)^{r-m}}{m!\,(r-m)!}\,\frac1{z-m}\,. $$ 
\endproclaim\bb{Proof} Compare residues on the two sides. \endpf
\proclaim{Lemma 2} Let $z$ and $y$ be two free variables.  Then
  $$\sum_{r=0}^\infty\frac{y^r}{z(z-1)\cdots(z-r)}
     \=e^{-y}\,\sum_{m=0}^\infty\frac{y^m}{m!}\,\frac1{z-m}\,. $$ 
\endproclaim\bb{Proof} The equality of the coefficients of $y^r$ is Lemma 1.  Alternatively, we
can prove the identity directly by observing that it holds for $y=0$ and that
  $$\align\frac \partial{\partial y}\bigl(y^{-z}\,e^y\cdot\text{LHS}\bigr) &\=\sum_{r=0}^\infty
    \biggl(\frac{e^y\,y^{r-z}}{z\cdots(z-r)}\-\frac{e^y\,y^{r-z-1}}{z\cdots(z-r+1)}\biggr)\\
    &\=\,e^y\,y^{-z-1}\=\frac \partial{\partial y}\bigl(y^{-z}\,e^y\cdot\text{RHS}\bigr)\,.\qq\bs\endalign$$ 

We now prove several results saying that certain generating functions which are {\it a priori} power series are 
in fact polynomials.  We denote by $(x)_n$ the ascending Pochhammer symbol $x(x+1)\cdots(x+n-1)$.
\proclaim{Proposition 1} For each $n\ge0$, there is a unique polynomial $B_n(z,y,t)$ in three variables $z$,~$y$~and $t$, 
of degree $n-1$, satisfying the identity
  $$ (z-t)\,B_n(z,y,t)\-y\,B_n(z-1,y,t)\=(z)_n\-\sum_{m=0}^n\binom nmy^m(t)_{n-m}\,. \tag 17 $$
\endproclaim\bb{Examples} For $0\le n\le3$ the polynomials $B_n$ are given by
   $$B_0=0,\;B_1=1,\;B_2=z+y+t+1,\;B_3=(z+1)(z+2)+(y+t)(z+y+t)+y+3t\,.$$ 
\bb{Proof}  The recursion is equivalent to the functional equation
  $$ (z-t)\,\B(z,y,t,u)\-y\,\B(z-1,y,t,u)\=(1-u)^{-z}-e^{yu}(1-u)^{-t}\tag 18$$
for the generating function $\B(z,y,t,u)=\sum\limits_{n=0}^\infty B_n(z,y,t)\dfrac{u^n}{n!}\,$.
The solution of this is
  $$ \B(z,y,t,u)\=(1-u)^{-t}\,\B_0(z-t,y,u)\,,\tag 19$$
where $\B_0(z,y,u)$ ($=\B(z,y,0,u)$) satisfies the simpler functional equation
  $$z\,\B_0(z,y,u)\-y\,\B_0(z-1,y,u)\=(1-u)^{-z}\-e^{yu}\,.\tag 20$$
Write $\B_0(z,y,u)$ as $\sum_{r\ge0}\b_r(z,u)\,y^r\,$. Then (20) is equivalent to
  $$z\,\b_r(z)=\cases\;(1-u)^{-z}-1&\text{if $r=0$,}\\\b_{r-1}(z-1,u)\-\dfrac{u^r}{r!}&\text{if $r>0$,}\endcases$$
which can be solved by induction on $r$ to give the closed formula
  $$\b_r(z,u)\=\frac{(1-u)^{-z+r}}{z(z-1)\cdots(z-r)}
     \-\sum_{s=0}^r\frac1{z(z-1)\cdots(z-s)}\,\frac{u^{r-s}}{(r-s)!}\,.\tag 21 $$
Using Lemma~1 we can rewrite (21) as
 $$\b_r(z,u)\=\sum_{m=0}^r\frac{(-1)^{r-m}}{m!\,(r-m)!}\;\frac{(1-u)^{-z+r}\-(1-u)^{r-m}}{z-m}  $$
or, going back to the generating function $\B_0$, 
  $$\B_0(z,y,u)\=e^{y(u-1)}\,\sum_{m=0}^\infty\frac{y^m}{m!}\;\frac{(1-u)^{-z+m}\-1}{z-m}\,.\tag 22 $$
Substituting this into (19) gives the generating series $\B(z,y,t,u)$ in the form
  $$\B(z,y,t,u)\=e^{y(u-1)}\,\sum_{m=0}^\infty\frac{y^m}{m!}\;\frac{(1-u)^{-z+m}\-(1-u)^{-t}}{z-m-t}\,.\tag 23$$
To see that the coefficients of this with respect to $u$ are polynomials, we rewrite (22) as
  $$\align \B_0(z,y,u)&\=e^{y(u-1)}\,\sum_{m=0}^\infty\frac{y^m}{m!}\;\int_0^u(1-v)^{-z+m-1}\,dv\\
   &\=\int_0^u(1-v)^{-z-1}\,e^{y(u-v)}\,dv\tag 24\\
    &\=\sum_{p=0}^\infty\sum_{q=0}^\infty\frac{(z+1)_p\,y^q}{p!\,q!}\,\int_0^uv^p(u-v)^q\,dq\\
    &\=\sum_{p=0}^\infty\sum_{q=0}^\infty\frac{(z+1)_p\,y^q\,u^{p+q+1}}{(p+q+1)!}\endalign$$
(the last equality by Euler's beta integral). Now substituting this into (19) and using the binomial expansion
of $(1-u)^{-t}$ gives the explicit polynomial expression
  $$ B_n(z,y,t)\=\sum\Sb p,\,q,\,l\ge0\\p+q+l+1=n\endSb\binom nl\,(z-t+1)_p\,(t)_l\,y^q\;\in\,\Z[z,y,t]\,. \qq\bs \tag 25$$

Of course, we could have simply written down (25) and checked that it satisfies the identity (17); we gave the
full derivation for clarity and because some of the formulas found along the way will be needed below.  In particular,
from (24) and (19) we get the integral representation
 $$\B(z,y,t,u)\=(1-u)^{-t}\,\int_0^u(1-v)^{-z+t-1}\,e^{y(u-v)}\,dv\tag 26$$
and from (21) and (19), or (23) and Lemma~2, we get the generating function identity
 $$\B(z,y,t,u)=\sum_{r=0}^\infty\frac{(1-u)^{-z+r}\,y^r}{(z-t)\cdots(z-t-r)}
      \-(1-u)^{-t}\,e^{uy}\,\sum_{r=0}^\infty\frac{y^r}{(z-t)\cdots(z-t-r)}\,.\tag 27$$
This can also be obtained from (26) by writing $\int_0^u=-\int_u^1+\int_0^1\,$ (for $\Re(z-t)<0$). 

\newpage
We now consider the specialization of the above functions to the case $y=-t$.  
 \proclaim{Proposition 2} For each $n\ge0$, there is a unique polynomial $\wB_n(z,t)$ in $z$~and $t$, of
 degree $[(n-1)/2]$ in $t$, satisfying the identity
  $$ (z-t)\,\wB_n(z,t)\+t\,\wB_n(z-1,t)\=(z)_n\-\sum_{m=0}^n\binom nm(-t)^m(t)_{n-m}\,. \tag 28 $$
\endproclaim\bb{Examples} For $0\le n\le4$ we have
   $$\wB_0=0,\;\wB_1=1,\;\wB_2=z+1,\;\wB_3=2t+(z+1)_2\,,\;\wB_4=3(z+3)t+(z+1)_3\,.$$ 
\bb{Proof} Since (28) is just the specialization of (17) to $y=-t$, its solution is of course given simply 
by $\wB_n(z,t)=B_n(z,-t,t)\,$; what we have to show is that the degree with respect to~$t$ drops by a factor 
of~2 under this specialization.  To do this we expand $(1-v)^{-z-1}$ in the integral representation (26) 
by the binomial theorem and change $v$ to $uv$ to get
 $$ \B(z,-t,t,u)\=\sum_{r=0}^\infty\binom{z+r}r\,u^{r+1}\,\int_0^1v^r\,\biggl[\frac{1-uv}{1-u}\,e^{uv-u}\biggr]^t\,dv\,.$$
The expression in square brackets has a power series expansion in $u$ beginning $1+\text O(u^2)$, so the integrand
is a power series in $tu^2$ and $u$.  It follows that $\B(z,-t,t,u)$ is $u$ times a power series in $tu^2$ and $u$
and hence that the coefficient $\wB_n(z,t)$ of $u^n$ has degree $\le(n-1)/2$ in $t$ for every $n$, as claimed.
Specifically, from the expansion 
 $$\frac{1-uv}{1-u}\,e^{uv-u}\=\exp\biggl(\sum_{m=2}^\infty\frac{u^m}m\,(1-v^m)\biggr)$$
we find the closed form
$$\wB_n(z,t)\,=\!\sum\Sb r,\,k_2,\,k_3,\ldots\ge0\\ r+2k_2+3k_3+\cdots=n-1\endSb\!\binom{z+r}r\,
   \frac{t^{k_2+k_3+\cdots}}{2^{k_2}k_2!\,3^{k_3}k_3!\,\cdots}\,\int_0^1v^r(1-v^2)^{k_2}(1-v^3)^{k_3}\cdots\,dv$$
from which the coefficients of $\wB_n$ can be computed explicitly. In particular, we see that $l+2m\le n-1$ for all monomials 
$z^lt^m$ occurring in $\wB_n$, and that in the case of equality the coefficient of this monomial comes only from the term 
$r=l$, $k_2=m$, $k_3=k_4=\cdots=0$ in the above sum and equals the beta integral $\int_0^1v^l(1-v^2)^mdv/2^ml!m!$. \endpf

Now comes the second point.  The specialization $y=-t$ had the effect in the above proof of making the linear term in
the power series expansion of $\,\bigl(\frac{1-uv}{1-u}\bigr)^te^{-uy(1-v)}\,$ vanish, but it also has a second, less
obvious effect:  if we denote by $U(x)$ the power series
 $$ U(x)\: 1-\frac x{e^x-1}\=\frac x2\-\frac{x^2}{12}\+\frac{x^4}{720}\-\cdots\;, $$
then we have
 $$ u=U(x)\q\Longrightarrow\q\frac{e^{-u}}{1-u} \= \frac{e^x-1}{xe^{x/2}}\,\exp\biggl(\frac x{e^x-1}+\frac x2-1\biggr)\=F(x)\,,\tag 29$$
where $F(x)$ is the power series defined in Theorem~4 in \S1 and is an {\it even} function of $x$.  This leads 
immediately to the following definition and proposition:
\proclaim{Proposition 3} For each positive integer $g$, the function  
  $$ P_g(z,t)\: \C{x^{2g-1},\,\B\bigl(z,-t,t,U(x)} \tag 30$$
is a polynomial of degree $2g-2$ in $z$ and $g-1$ in $t$ and satisfies the identities
    $$ (z-t)\,P_g(z,t)\+t\,P_g(z-1,t)\=S_{2g-1}(z) \tag 31$$
and
   $$ P_g(z,t)\=\sum_{r=0}^\infty \frac{S_{2g-1}(z-r)\,(-t)^r}{(z-t)\cdots(z-t-r)}\q\in\;\Q(z)[[t]]\,.\tag 32$$
\endproclaim
\bb{Proof} Equation (31) follows by substituting $y=-t$, $u=U(x)$ into the generating series identity (18),
since the second term $e^{-tu}(1-u)^{-t}$ on the right is an even power series in $x$ by virtue of
equation (29), while the coefficient of $x^{2g-1}$ in the first term $(1-u)^{-z}$ is $S_{2g-1}(z)$ by definition.
Similarly, equation (32) is obtained by substituting $y=-t$, $u=U(x)$ into (27) and noting that the second term
is an even power series in $x$.\endpf

\bigskip {\bf 3. Proof of Theorems 2--5.} We begin with Theorem~2. From (3) and (7) we have
$$ A(g,n)\=\sum_{1\le l\le k\le n}\frac{(-1)^{n-k}\,k^{-l-1}}{(n-k)!\,(k-l)!}\,S_{2g-1}(l)\,.$$
For fixed $l$ the coefficient of $S_{2g-1}(l)$ can be rewritten
$$ \align \sum_{k=l}^n\frac{(-1)^{n-k}}{(n-k)!\,(k-l)!}\,k^{-l-1}
   &\=\C{t^l,\;\sum_{k=l}^n\frac{(-1)^{n-k}}{(n-k)!\,(k-l)!}\,\frac1{k-t}} \\
   &\=\C{t^l,\;\frac{(-1)^{n-l}}{(n-t)(n-t-1)\cdots(l-t)}} \endalign $$
(the latter by Lemma~1 with $r=n-l$, $z=n-t$), so, replacing $l$ by $r=n-l$,
$$  A(g,n)\=\C{t^n,\;\sum_{r=0}^{n-1}\frac{S_{2g-1}(n-r)\,(-t)^r}{(n-t)(n-t-1)\cdots(n-r-t)}}\,.\tag 33$$
The key observation is now that if we replace the summation on the right by one from $r=0$~to~$\infty$, then its value does not change: 
the terms $r=n$ and $r=n+1$ contribute nothing because $S_{2g-1}(0)=S_{2g-1}(-1)=0$, and the terms with $r\ge n+2$
contribute nothing because the rational function $1/(n-t)(n-t-1)\cdots(n-t-r)$ has only a simple pole at $t=0$ and hence
its product with $t^r$ has no coefficient of $t^n$.  Hence equation (32) gives
$$  A(g,n)\=\C{t^n,\,P_g(n,t)}\,.$$
This proves the vanishing of $A(g,n)$ for $n\ge g$ (since $P_g(z,t)$ is a polynomial of degree $\le g-1$ in $t$ for all $z$)
and hence also the fact that $P_g(k)$ is a polynomial in $k$ of degree $g-1$.  The statement (4) about the values of the
numbers $A(g,n)$ for $g-n$ fixed can be proved by using the integral representation of the generating function
$\B(z,-t,t,u)$, but since the argument is similar to the one we give below for equation (2) (to which (4) is in fact 
equivalent), and since the statement about the form of the $A(g,n)$ was included only for amusement, we omit the derivation.

We now turn to $A_\nu(g,n)$. The same argument as was used to derive (33) gives
$$  A_\nu(g,n)\=\C{t^{n+\nu},\;\sum_{r=0}^{n-1}\frac{S_{2g-1}(n-r)\,(-t)^r}{(n-t)(n-t-1)\cdots(n-r-t)}}$$
for any $\nu>0$, but now changing the sum to one over all $r\ge0$ does change the right-hand side,
since the terms $r=n+\mu+1$ of the sum have non-0 coefficients of $t^n$ for $1\le\mu\le\nu$. Equation (32) therefore now gives  
$$  A_\nu(g,n)\=\C{t^{n+\nu},\,P_g(n,t)}\-\C{t^\nu,\,\frac{(-1)^n}{(n-t)\cdots(1-t)}\,
  \sum_{\mu=1}^\nu\frac{S_{2g-1}(-\mu-1)\,t^\mu}{(1+t)\cdots(\mu+1+t)}}\,.$$
Again the first term vanishes for $n$ sufficiently large ($n\ge g-\nu$), so for small $\nu$ we get explicit formulas
for $\nu$, two examples being given by equation (5).  By analyzing these formulas we could deduce the statement in part~(iii)
of Theorem~1 about the lowest coefficients of $P_g(k)$. But it will be easier to work directly with $P_g(k)$, using the following result. 

\proclaim{Proposition 4} For each positive integer $k$ the polynomials $P_g(z,t)$ defined by $(30)$ satisfy the identity
 $$ P_g(t-k,t)\=\sum_{l=1}^k\frac{(k-1)!}{(k-l)!}\,t^{-l}\,S_{2g-1}(l+t-k)\,.   \tag 34$$
In particular, the function $P_g(k)$ defined by $(1)$ is equal to the polynomial $P_g(0,k)$. \endproclaim
\bb{Proof} We prove this by induction on $k$: setting $z=t$ in (31) gives the case $k=1$ of (34), and
setting  $z=t-k$ in (31) gives the induction step from $k$ to $k+1$.\endpf

The remaining results stated in \S1 follow easily from the last statement of Proposition~4. Theorem 3 is obtained immediately by 
taking $z=0$ in equation (32). For Theorem~4, we first use the integral representation (26) to write
$$ \B(0,-t,t,u)\=\biggl(\frac{e^{-u}}{1-u}\biggr)^t\,\int_0^u\biggl(\frac{e^{-v}}{1-v}\biggr)^{-t}\,\frac{dv}{1-v}\,.$$
Now making the substitutions $u=U(x)$ and $v=U(y)$ and using equation (29) we get
$$ \B(0,-t,t,U(x))\=F(x)^t\,\int_0^xF(y)^{-t}\,\frac{U'(y)}{1-U(y)}\,dy\,.$$
But
$$\frac{U'(y)}{1-U(y)}\=\frac{e^y}{e^y-1}\-\frac1y\=\frac12\+\text{(odd power series in $y$)}\,,$$
so
$$ \B(0,-t,t,U(x))\=\frac12\,F(x)^t\,\int_0^xF(y)^{-t}\,dy\+\text{(even power series in $x$)}\,.$$
Equation (10) now follows from the equality $P_g(t)=P_g(0,t)$ and the definition of $P_g(z,t)$.  
Finally, the recursion (11) is, as already stated in \S1, equivalent to equation (10): if we denote by
$\P(x,t)$ the generating function occurring on the left-hand side of~(10), then 
$$ (10)\q\Longleftrightarrow\q \frac12\=F(x)^t\,\frac{\partial}{\partial x}\bigl(F(x)^{-t}\,\P(t,x)\bigr)
  \=\frac{\partial\P(x,t)}{\partial x}\-t\,\frac{F'(x)}{F(x)}\,\P(t,x)\,,\tag 35$$
and this is seen to be equivalent to (11) by substituting $F'(x)/F(x)=\sum_{n\ge1}(2n+1)\b_{2n}x^{2n-1}$
from (9) and comparing the coefficients of $x^{2g-2}$ on both sides.

\bigskip {\bf 4. Proof of Theorem 1.}  We now know, from Proposition~4 or Theorem~4 or~5, that $P_g(k)$ is
a polynomial. It remains to prove the statements made in Theorem~1 about the coefficients $c_{g,g-j-1}$ 
($j$ fixed) and $c_{g,i}$ ($i$ fixed). We start with the ``top" coefficients $c_{g,g-j-1}$. Writing $y=vx$ in (10)  we find
   $$  \sum_{g=1}^\infty P_g(t)\,x^{2g-2}=\frac12\,\int_0^1
     \,\exp\biggl(\sum_{r=1}^\infty \l_r\,tx^r(1-v^r)\biggr)\,dv$$
where $\l_r=\C{x^{2r},\,\log F(x)}=(1+1/2r)\,\b_{2r}\,$.  Expanding the integral 
as in the proof of Proposition~2 and comparing the coefficients of $x^{2g-2}t^{g-j-1}$ on both sides, we find
$$ \align c_{g,g-j-1}&\=\frac12\,\sum\Sb\a,\,\b,\,\g\,\cdots\ge0\\ \a+2\b+3\g+\cdots=g-1\\ \b+2\g+\cdots=j\endSb
   \frac{\l_1^\a}{\a!}\,\frac{\l_2^\b}{\b!}\,\frac{\l_3^\g}{\g!}\cdots\,\int_0^1(1-v^2)^\a(1-v^4)^\b(1-v^6)^\g\,\cdots\,dv \\
  &\= \frac12\sum_{j\le d\le2j}\,\frac{\l_1^{g-d-1}}{(g-d-1)!}\,\int_0^1(1-v^2)^{g-j-1}\,H_{j,d}(v^2)\,dv  \endalign $$
with
$$  H_{j,d}(x)\=\sum\Sb\a,\,\b,\,\g\,\cdots\ge0\\ \b+2\g+\cdots=j\\ 2\b+3\g+\cdots=d\endSb 
   \frac{\l_2^\b}{\b!}\,\frac{\l_3^\g}{\g!}\cdots\,(1+x)^\b\,(1+x+x^2)^\g\cdots \;.$$
This can now be computed by expanding $H_{j,d}$ as a polynomial and computing each term
$\int_0^1(1-v^2)^{g-j-1}v^{2n}dv$ as a beta integral, and can easily be seen to have the form (2) for some polynomial
$C_j(g)$. The highest power of $g$ occurs for the maximal value $d=2j$, corresponding to taking $\b=j$ and $\g=\cdots=0$.
Also, to compute the coefficient of the highest power of $g$ we may replace $H_{j,d}(x)$ by its constant term $H_{j,d}(0)$,
since the main contribution to the integral for $g$ large comes from $v$ near 0, and the asymptotic value of
$\int_0^1(1-v^2)^{g-j-1}\,dv$ is $C(g)=2^{2g-2}(g-1)!^2/(2g-1)!$ (independent of $j$) by the beta integral formula.
It follows that the asymptotic formula for $c_{g,g-j-1}$ is
$$ c_{g,g-j-1}\,\sim\,\frac{C(g)}2\,\frac{\l_1^{g-2j-1}}{(g-2j-1)!}\,\frac{(2\l_2)^j}{j!}
\,\sim\,\frac{C(g)\l_1^{g-1}}{2(2g-1)!}\;g^{2j}\;\frac{(2\l_2/\l_1^2)^j}{j!}\,,$$
and this agrees with the result stated in Theorem~1 because $\l_1=1/8$ and $2\l_2/\l_1^2=-2/9\,$.  One can also
prove equation (2), and obtain explicit recursion relations for the polynomials $C_j(g)$, from the recursion relation
given in Theorem 5. The details are left to the reader.

For the ``bottom" coefficients $c_{g,i}$ ($i$ fixed) we use the expansion (8) together with the following lemma,
which expresses the ``negative Stirling numbers" $S_n(-r)$ for $r$ fixed as finite linear combinations of Bernoulli numbers:
\proclaim{Lemma 3}  For $n\ge r\ge1$ we have the identity
$$ S_n(-r) \= \sum_{j=0}^{r-1}(-1)^{r-1-j}\binom{n-j-1}{r-j-1}\,S_j(-r)\,\b_{n-j}\,.$$
\endproclaim 
\bb{Proof} One sees by induction that the powers of the function $1/(e^x-1)$ are linear combinations of its
derivatives.  From the formulas
$$ \biggl(\frac1{e^x-1}\biggr)^r\=\sum_{s=1}^r\,S_{r-s}(-r)\,\frac1{x^s}\+\text O(1)\qq\qq(x\to0)$$
and 
$$ \frac{(-1)^{s-1}}{(s-1)!}\,\frac{d^{s-1}}{dx^{s-1}}\biggl(\frac1{e^x-1}\biggr)
  \=\frac1{x^s}+(-1)^{s-1}\sum_{l=s}^\infty\binom{l-1}{s-1}\,\b_l\,x^{l-s}$$
we deduce 
$$ \biggl(\frac1{e^x-1}\biggr)^r\=\sum_{s=1}^r\,S_{r-s}(-r)\,
\biggl(\frac1{x^s}+(-1)^{s-1}\sum_{l=s}^\infty\binom{l-1}{s-1}\,\b_l\,x^{l-s}\biggr)\,,$$
and the desired result follows by comparing coefficients of $x^{n-r}$ on both sides.\endpf

Part (iii) of Theorem~1 follows immediately from (8) and Lemma~3.  Explicitly, we have
  $$ c_{g,i}\=\sum_{j=0}^i\biggl(\sum_{r=j+1}^{i+1}(-1)^{r-j}\,\binom{2g-j-2}{r-j-1}\,S_j(-r)\,\a_{i-r+1}(r)\biggr)\,\b_{2g-j-1}\,,$$
where
  $$ \a_n(r) \: \C{t^n,\,\frac1{(1+t)\cdots(r+t)}}\=\frac{(-1)^n}{r!}\,h_n\bigl(1,\,\frac12,\ldots,\,\frac1r\bigr)\,,\tag 36$$
and the coefficient of $\b_{2g-j-1}$ in this formula is a polynomial of degree $i-j$ in $g$. \endpf

\bigskip {\bf 5. The polynomials $Q_i(y)$ and the second generating function for the $c_{g,i}$.}  In this section we will discuss the 
polynomials defined by equations (12)--(14) and prove Theorem~6.  We must first check that the power series in (12) is indeed a 
polynomial of degree $i+1$ and that the three definitions are indeed equivalent.  For the first statement, note that if $n\ge i+2$ then 
$$ \C{y^n,\,Q_i(y)} \= \sum_{k=1}^n\frac{k^{k-1-i}}{k!}\cdot\frac{(-k)^{n-k}}{(n-k)!}\=\frac1{n!}\,\sum_{k=0}^n(-1)^{n-k}\binom nk\,k^{n-1-i}\=0$$
(the $n$th difference of a polynomial of degree $<n$ vanishes).  For the second, note that the system of integral recursions (13) is 
equivalent to the system of differential recursions
$$ Q_0(y)=y\,,\qq y\,Q_{i+1}'(y)=(y-1)\,Q_i(y)\qq(i\ge0)\tag 37$$
(no initial values are needed here because the ($i+1$)st equation in this system implies that $Q_{i+1}(0)=0$, which is the needed initial
condition to solve the $i$th equation).  It is easy to check that the functions satisfied by (12) or by (14) both satisfy
the system (37), so they are all equal.  We can write out (14) more explicitly as 
$$ Q_i(y)\=\sum_{r=1}^{i+1}\a_{i+1-r}(r)\,y^r\,, \tag 38$$ 
with $\a_n(r)$ defined by  (36); these numbers obviously satisfy  $\a_n(r-1)=r\a_n(r)+\a_{n-1}(r)$,
and this is equivalent to the statement that the polynomials given in (38) satisfy (37). 

Now set $Y(x)=x/(1-e^{-x})$ and $\tQ_i(x)=Q_i(Y(x))$.  Then (37) gives
$$ \tQ_{i+1}'(x)\=Y'(x)\,\frac{Y(x)-1}{Y(x)}\,\tQ_i(x)\;=:\;\g(x)\,Q_i(x)\,.\tag 39$$
But an easy calculation shows that the function $\g(x)$ is nothing other than the logarithmic derivative $F'(x)/F(x)$
of the function defined in (9). In particular it is an {\it odd} function of~$x$, so that from (39) we deduce that also
$$ \frac d{dx}\bigl(\tQ_{i+1}(x)\-\tQ_{i+1}(-x)\bigr)\= \g(x)\,\bigl(\tQ_i(x)\-\tQ_i(-x)\bigr)  \,.\tag 40$$
This equation and the fact that $\tQ_i(x)-\tQ_i(-x)$ vanishes at $x=0$ imply by induction on~$i$ that $\tQ_i(x)-\tQ_i(-x)$ 
vanishes to order $2i+1$ at the origin for all $i\ge0$, which is the first assertion of Theorem~6.  (The uniqueness statement
follows immediately from the existence since the polynomials $Q_0,\,Q_1,\ldots,Q_i$ form a basis for the space of polynomials
of degree $\le i+1$ with no constant term.)  Equation (16), which can be written as the generating function identity
$$ 2\,\sum_{g=1}^\infty P_g(t)\,x^{2g-1}\=\sum_{i=0}^\infty\bigl(\tQ_i(x)\-\tQ_i(-x)\bigr)\,t^i\,,\tag41$$
follows at the same time, since the differential equation (40) is equivalent to the differential equation in (35) for
the generating series $\sum P_g(t)\,x^{2g-1}$ or to the recursion (11) for its coefficients. \endpf

\bigskip \bigskip
[1] C.~Faber and R.~Pandharipande, {\it Logarithmic series and Hodge integrals in the tautological ring}, this volume, pp.~XX--XX.

\end
